# Supplementary material for: Late Time Acceleration with Observational Constraints in Modified Theories of Gravity
Source: arXiv:2401.00054 source file (2023-12-29)
Supplement: Supplementary file 2 [file sample-si.tex]

% This file is public domain
% If you want to use arara, you need the following directives:
% arara: pdflatex: { synctex: on }
% arara: makeglossaries
% arara: pdflatex: { synctex: on }
%
%http://mirrors.ctan.org/macros/latex/contrib/glossaries/glossaries-user.html#sample-si
\documentclass{article}
\usepackage{siunitx}
\usepackage[style=long4col]{glossaries}

\makeglossaries

\newglossaryentry{ohm}{%
  name=ohm,
  symbol={\si{\ohm}},
  description=unit of electrical resistance%
}

\begin{document}
\glsaddallunused

\printglossaries
\end{document}
